# Supplementary material for: Correlated Fractional Dirac Materials
Source: arXiv:2207.09449 ancillary file (2023-07-10)
Supplement: Supplementary file 1 [file Supplementary_FDM.pdf]

# Supplementary Materials: Correlated Fractional Dirac Materials


Bitan Roy[1] and Vladimir Juričić[2,3]

[1]Department of Physics, Lehigh University, Bethlehem, Pennsylvania, 18015, USA

[2]Departamento de Física, Universidad Técnica Federico Santa María, Casilla 110, Valparaíso, Chile

[3]Nordita, KTH Royal Institute of Technology and Stockholm University, Hannes Alfvéns väg 12, 106 91 Stockholm, Sweden



(Dated: January 28, 2023)



The Supplementary Materials contain derivation of the (a) density of states [Sec. S1] and (b) optical conductivity [Sec. S2] in fractional Dirac materials (FDMs). In addition, we also display details of (c) the renormalization group (RG) calculation of the Gross-Neveu model [Sec. S3], (d) derivation of the self-consistent mean-field gap equation of the chiral symmetry breaking mass generation [Sec. S4] and (d) RG calculation with long range Coulomb repulsion [Sec. S5] in FDMs


## S1. DENSITY OF STATES IN FDM

The density of states (DOS) of a $d$-dimensional FDM at energy $E$ is defined as

$$\varrho(E) = D \int \frac{d^d \boldsymbol{k}}{(2\pi)^d} \, \delta\left(E - E_\alpha(\boldsymbol{k})\right), \tag{S1}$$

where $\delta(x)$ is the Dirac delta function of its argument $x$, $D$ is the dimensionality of the mutually anticommuting $\Gamma$ matrices appearing in Eq. (1) of the main text and $E(\boldsymbol{k})$ is the energy spectra of a FDM of order $\alpha$ given by

$$E_\alpha(\boldsymbol{k}) = v_\alpha \left[ \sum_{j=1}^{d} |k_j|^{2\alpha} \right]^{1/2} \equiv v_\alpha |k|^\alpha \left[ \sum_{j=1}^{d} |\hat{\Omega}_j|^{2\alpha} \right]^{1/2}. \tag{S2}$$

Here $\hat{\Omega}_j$ are the components of a $d$-dimensional spherical unit vector. The identity involving the delta function reads

$$\delta(E - E_\alpha(\boldsymbol{k})) = \frac{\delta(k - k_0)}{|E'_\alpha(k_0)|}, \tag{S3}$$

where prime ($'$) denotes derivative and $k_0$ is determined from the relation $E = E_\alpha(\boldsymbol{k}_0)$, which more explicitly reads

$$E = v_\alpha k_0^\alpha \left[ \sum_{j=1}^{d} |\hat{\Omega}_j|^{2\alpha} \right]^{1/2} \Rightarrow k_0 = \frac{E^{1/\alpha}}{v^{1/\alpha} \left[ |\hat{\Omega}_j|^{2\alpha} \right]^{1/(2\alpha)}} \Rightarrow E'_\alpha(k_0) = \alpha \, v_\alpha^{1/\alpha} \, E^{1-\alpha^{-1}} \, [f(\hat{\Omega})]^{1/(2\alpha)}, \tag{S4}$$

where $f(\hat{\Omega}) = \sum_{j=1}^{d} |\hat{\Omega}_j|^{2\alpha}$. With these simplifications, the DOS can be compactly written as

$$\varrho(E) = |E|^{\frac{d}{\alpha}-1} \left( \frac{D}{v_\alpha^{d/\alpha}} \right) \int \frac{d\Omega}{(2\pi)^d} \, \frac{1}{\alpha [f(\hat{\Omega})]^{d/(2\alpha)}} \equiv |E|^{\frac{d}{\alpha}-1} \, D_d(\alpha). \tag{S5}$$

For $\alpha = 1$ we immediately recover the known scaling forms of conventional Dirac systems in two and three dimensions. The scaling of the functions $D_2(\alpha)$ and $D_3(\alpha)$ are shown in Fig. 2(a) and (b) of the main text.

## S2. OPTICAL CONDUCTIVITY IN FDM

The diagonal component of the optical conductivity (OC) at a (real) frequency $\Omega$ is defined as

$$\sigma_{jj}(\Omega) = -\frac{\Im \, \Pi_{jj}(i\Omega \to \Omega + i\delta)}{\Omega} \tag{S6}$$

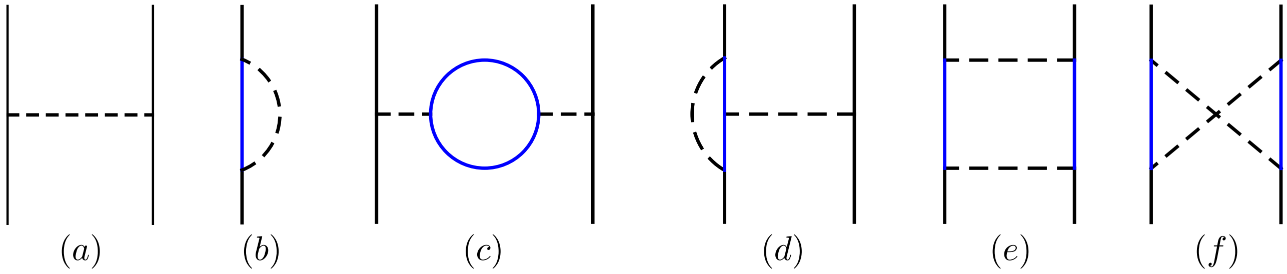

Figure S1. (a) Bare four-fermion interaction vertex and (b) the self-energy correction due to four-fermion interaction. The contribution from the Feynman diagram (b) is identically zero. Feynman diagrams (c)-(f) yield corrections to the bare interaction vertex to the leading order in the $\epsilon$ expansion, where $\epsilon = d - \alpha$. Here, solid lines represent fermions. The blue lines in (b)-(f) correspond to the fast modes, living within a thin Wilsonian momentum shell $\Lambda\, e^{-\ell} < |\boldsymbol{k}| < \Lambda$ and the black lines represent the slow modes with $|\boldsymbol{k}| < \Lambda\, e^{-\ell}$. Here $\Lambda$ is the ultraviolet momentum cut-off and $\ell$ is the logarithm of the RG scale.

where the associated polarization tensor is defined through the corresponding current-current correlator as

$$\Pi_{jm}(i\Omega) = \mathrm{Tr} \int_{-\infty}^{\infty} \frac{d\omega}{2\pi} \int \frac{d^d\boldsymbol{k}}{(2\pi)^d} \left\{ J_j(\boldsymbol{k}) G_0(i\omega + i\Omega, \boldsymbol{k}) J_m(\boldsymbol{k}) G_0(i\omega, \boldsymbol{k}) \right\} \tag{S7}$$

where $\omega$ is the fermionic Matsubara frequency and $j, m = 1, \cdots, d$. The Green function and the current operator are respectively defined as

$$G_0(i\omega, \boldsymbol{k}) = \frac{1}{i\omega - H_{\mathrm{FD}}(\boldsymbol{k})} = -\frac{i\omega + H_{\mathrm{FD}}(\boldsymbol{k})}{\omega^2 + E_\alpha^2(\boldsymbol{k})} \quad \text{and} \quad J_j(\boldsymbol{k}) = \frac{\partial H_{\mathrm{FD}}(\boldsymbol{k})}{\partial k_j} = \alpha v_\alpha |k_j|^{\alpha-1} \Gamma_j. \tag{S8}$$

The explicit form of $H_{\mathrm{FD}}(\boldsymbol{k})$ is shown in Eq. (1) of the main manuscript.

Next we show the detailed derivation of $\sigma_{xx}(\Omega)$. We arrive at same conclusions for the components of the OC along the other principal axes. Specifically,

$$\begin{aligned}
\Pi_{xx}(i\Omega) &= \mathrm{Tr} \int_{-\infty}^{\infty} \frac{d\omega}{2\pi} \int \frac{d^d\boldsymbol{k}}{(2\pi)^d}\, \alpha^2 v_\alpha^2 |k_x|^{2(\alpha-1)} \left\{ \Gamma_1 \, \frac{i(\omega+\Omega) + H_{\mathrm{FD}}(\boldsymbol{k})}{(\omega+\Omega)^2 + E_\alpha^2(\boldsymbol{k})} \, \Gamma_1 \, \frac{i\omega + H_{\mathrm{FD}}(\boldsymbol{k})}{\omega^2 + E_\alpha^2(\boldsymbol{k})} \right\} \\
&= D \int_{-\infty}^{\infty} \frac{d\omega}{2\pi} \int \frac{d^d\boldsymbol{k}}{(2\pi)^d}\, \alpha^2 v_\alpha^2 |k_x|^{2(\alpha-1)} \, \frac{-\omega(\omega+\Omega) + v_\alpha^2 \left\{ |k_x|^{2\alpha} - \sum_{j=2}^{d} |k_j|^{2\alpha} \right\}}{(\omega^2 + E_\alpha^2(\boldsymbol{k}))([\omega+\Omega]^2 + E_\alpha^2(\boldsymbol{k}))} \\
&= D \int \frac{d^d\boldsymbol{k}}{(2\pi)^d}\, \alpha^2 v_\alpha^2 |k_x|^{2(\alpha-1)} \left[ \frac{-2 v_\alpha^2 \sum_{j=2}^{d} |k_j|^{2\alpha}}{[\Omega^2 + 4E_\alpha^2(\boldsymbol{k})] E_\alpha(\boldsymbol{k})} \right] = -2D\alpha^2 v_\alpha^3 \int \frac{d^d\boldsymbol{k}}{(2\pi)^d} \, \frac{k^{3\alpha-2} |\Omega_x|^{2\alpha-2} \sum_{j=2}^{d} |\Omega_j|^{2\alpha}}{\sqrt{f(\hat{\Omega})} \left[ \Omega^2 + 4 v_\alpha^2 f(\hat{\Omega}) k^{2\alpha} \right]}.
\end{aligned} \tag{S9}$$

After the analytic continuation $i\Omega \to \Omega + i\delta$ to the real frequency $\Omega$ and using the identity

$$\frac{1}{(\Omega + i\delta)^2 - 4v_\alpha^2 f(\hat{\Omega}) k^{2\alpha}} = \frac{1}{2v_\alpha \sqrt{f(\hat{\Omega})} k^\alpha} \left( \frac{1}{\Omega + i\delta - 2v_\alpha \sqrt{f(\hat{\Omega})} k^\alpha} - \frac{1}{\Omega + i\delta - 2v_\alpha \sqrt{f(\hat{\Omega})} k^\alpha} \right), \tag{S10}$$

such that for $\Omega > 0$, for example, only the first term contributes, which after taking the limit $\delta \to 0$ yields

$$\frac{1}{4v_\alpha \sqrt{f(\hat{\Omega})} k^\alpha} \, (-i\pi) \, \delta\left( \Omega - 2v_\alpha \sqrt{f(\hat{\Omega})} k^\alpha \right). \tag{S11}$$

Then the imaginary part of the polarization reads as

$$\begin{aligned}
\Im \Pi_{xx}(\Omega) &= -\frac{2\pi D \alpha^2 v_\alpha^2}{4} \int_0^\infty k^{d-1} dk \int \frac{d\hat{\Omega}}{(2\pi)^d} \, \frac{k^{2\alpha-2} |\Omega_x|^{2\alpha-2}}{f(\hat{\Omega})} \sum_{j=2}^{d} |\Omega_j|^{2\alpha} \; \delta\left( \Omega - 2v_\alpha \sqrt{f(\hat{\Omega})} k^\alpha \right) \\
&= -\frac{2D\pi\alpha v_\alpha}{8} \left( \frac{\Omega}{2v_\alpha} \right)^{1 + \frac{d-2}{\alpha}} \int \frac{d\hat{\Omega}}{(2\pi)^d} \, \frac{|\Omega_x|^{2\alpha-2}}{[f(\hat{\Omega})]^{5/2 + (d-2)/(2\alpha)}} \sum_{j=2}^{d} |\Omega_j|^{2\alpha}.
\end{aligned} \tag{S12}$$

The diagonal component of the OC along the $x$ direction in the units of $e^2/h$ then reads

$$\sigma_{xx}(\Omega) = \frac{e^2}{h} \frac{4D\pi^2 \alpha v_\alpha^2}{8(2v_\alpha)^{1+(d-2)/\alpha}} (\Omega)^{\frac{d-2}{\alpha}} \int \frac{d\hat{\Omega}}{(2\pi)^d} \frac{|\Omega_x|^{2\alpha-2}}{[f(\hat{\Omega})]^{5/2+(d-2)/(2\alpha)}} \sum_{j=2}^{d} |\Omega_j|^{2\alpha} \equiv \frac{e^2}{h} \frac{\pi D}{16} \left(\frac{\Omega}{v_\alpha}\right)^{\frac{d-2}{\alpha}} C_d(\alpha). \quad \text{(S13)}$$

The scaling of the universal function $C_d(\alpha)$ is shown in Fig. 2(c) and (d) of the main manuscript for $d = 2$ and 3. For conventional Dirac fermions ($\alpha = 1$) we recover the known results for the OC in $d = 2$ and 3, for which $C_2(1) = 1$ and $C_3(1) = 2/(3\pi)$.

## S3. DETAILS OF THE RG CALCULATION OF GROSS-NEVEU MODEL IN FDM

In this section we show the details of the leading order RG analysis for the four-fermion Gross-Neveu model for chiral symmetry breaking mass generation in FDMs, captured by the RG flow equation shown in Eq. (6) of the main text. The relevant Feynman diagrams are shown in Fig. S1. The contribution from the self-energy diagram is

$$(b) = g_m \int' \frac{d^d \boldsymbol{k}}{(2\pi)^d} \int_{-\infty}^{\infty} \frac{d\omega}{2\pi} G_0(i\omega, \boldsymbol{k}) \equiv 0. \quad \text{(S14)}$$

The integration over the spatial components of momentum is restricted within a thin Wilsonian shell $\Lambda\, e^{-\ell} < |\boldsymbol{k}| < \Lambda$ (denoted the 'prime' symbol), where $\Lambda$ is the ultraviolet momentum cutoff and $\ell$ is the logarithm of the RG scale. The contributions to the 'bubble' diagram (c) and 'vertex' diagram (d) are respectively given by

$$(c) = -2g_m^2 \,\mathrm{Tr} \int' \frac{d^d \boldsymbol{k}}{(2\pi)^d} \int_{-\infty}^{\infty} \frac{d\omega}{2\pi} \left[M G_0(i\omega, \boldsymbol{k}) M G_0(i\omega, \boldsymbol{k})\right] = g_m^2 D \,\frac{\Lambda^{d-\alpha}}{v_\alpha^d}\, \ell\, S_d(\alpha) \quad \text{(S15)}$$

$$\text{and} \quad (d) = \frac{4}{D} \mathrm{Tr} \left[M \int' \frac{d^d \boldsymbol{k}}{(2\pi)^d} \int_{-\infty}^{\infty} \frac{d\omega}{2\pi} M G_0(i\omega, \boldsymbol{k}) M G_0(i\omega, \boldsymbol{k}) M\right] = -2g_m^2 \,\frac{\Lambda^{d-\alpha}}{v_\alpha^d}\, \ell\, S_d(\alpha). \quad \text{(S16)}$$

The contributions from the remaining two Feynman diagrams (e) and (f) together take the form

$$(e) + (f) = 2g_m^2 \int' \frac{d^d \boldsymbol{k}}{(2\pi)^d} \int_{-\infty}^{\infty} \frac{d\omega}{2\pi} \left(\Psi_<^\dagger M G_0(i\omega, \boldsymbol{k}) \Psi_<\right) \Psi_<^\dagger \left(M G_0(i\omega, \boldsymbol{k}) M + M G_0(-i\omega, -\boldsymbol{k}) M\right) \Psi_< \equiv 0, \quad \text{(S17)}$$

where $\Psi_<^\dagger$ and $\Psi_<$ are the *slow* fermionic modes with momentum $|\boldsymbol{k}| < \Lambda e^{-\ell}$.

After collecting all these contributions, we arrive at the RG flow equation

$$\frac{dg_m}{d\ell} = (\alpha - d) g_m + (D-2) \frac{\Lambda^{d-\alpha}}{v_\alpha^d}\, S_d(\alpha)\, g_m^2. \quad \text{(S18)}$$

Upon multiplying both sides of the RG flow equation by $\Lambda^{d-\alpha} S_d(\alpha)/v_\alpha^d$, we can cast it in terms of the dimensionless coupling constant $\lambda_m = g_m \Lambda^{d-\alpha} S_d(\alpha)/v_\alpha^d$ as shown in Eq. (6) of the main text.

## S4. SOLUTION OF MEAN-FIELD GAP EQUATION IN FDM

In this section, we display the derivation of the mean-field free energy for the chiral symmetry breaking mass generation in FDMs. The partition function in a $d$-dimensional FDM interacting via short-range or local Gross-Neveu interaction ($g_m$) takes the form

$$\begin{aligned} \mathcal{Z} &= \int \mathcal{D}\Psi \mathcal{D}\Psi^\dagger \, \exp\left[i \int d^d\boldsymbol{x} d\tau \left\{ \Psi^\dagger \left[i\omega + H_{\rm FD}(\boldsymbol{k})\right] \Psi + g_m \left(\Psi^\dagger M \Psi\right)^2 \right\}\right] \\ &= \int \mathcal{D}\Psi \mathcal{D}\Psi^\dagger \mathcal{D}\Phi \, \exp\left[i \int d^d\boldsymbol{x} d\tau \left\{ \Psi^\dagger \left[i\omega + H_{\rm FD}(\boldsymbol{k}) - \Phi M\right] \Psi - \frac{N}{2g_m} \Phi^2 \right\}\right] \\ &= \int \mathcal{D}\Phi \, \exp\left[i \left\{ N \,\mathrm{Tr} \ln\left(i\omega + H_{\rm FD}(\boldsymbol{k}) - \Phi M\right) - \frac{N}{2g_m} \int d^d\boldsymbol{x} d\tau \Phi^2 \right\}\right]. \end{aligned} \quad \text{(S19)}$$

Here for brevity we set two independent Grassmann variables $\Psi(\boldsymbol{x},\tau) \equiv \Psi$ and $\Psi^\dagger(\boldsymbol{x},\tau) \equiv \Psi^\dagger$, and the real bosonic variable $\Phi(\boldsymbol{x},\tau) \equiv \Phi$. To arrive from the first to the second line, we performed a Hubbard-Stratonovich transformation of the four-fermion term (proportional to $g_m$) by introducing bosonic variable $\Phi$, yielding an action quadratic in fermionic fields. The last expression is obtained by integrating out the fermionic degrees of freedom. To proceed further, we now assume that $\Phi$ is independent of space ($\boldsymbol{x}$) and imaginary time ($\tau$). This restricts us to the mean-field approximation in which nontrivial $\Phi$ describes a uniform condensate of chiral-symmetry breaking Dirac mass. It can be determined from the self-consistent mean-field gap equation, which we derive next.

The corresponding mean-field free energy is then straightforwardly obtained from the above partition function, and is of the form

$$F = \frac{\Phi^2}{2g_m} - T\sum_{\omega_n}\int \frac{d^d\boldsymbol{k}}{(2\pi)^d}\,\mathrm{Tr}\ln\left(i\omega_n + H_{\mathrm{FD}}(\boldsymbol{k}) - \Phi M\right) = \frac{\Phi^2}{2g_m} - T\sum_{\omega_n}\int \frac{d^d\boldsymbol{k}}{(2\pi)^d}\ln(\omega_n^2 + E_\alpha^2(\boldsymbol{k}) + \Phi^2). \tag{S20}$$

Minimizing the free energy with respect to $\Phi$ we arrive at the gap equation shown in Eq. (9) of the main text.

## S5. RG ANALYSIS IN FDM WITH LONG RANGE COULOMB REPULSION

In this section, we show the detailed derivation of the RG flow equations in FDM in the presence of the long range repulsive Coulomb interaction. First we focus on the self-energy diagram which in $d$ dimensions reads as

$$\begin{aligned}\Sigma_d(i\Omega,\boldsymbol{k}) &= \int_{-\infty}^{\infty}\frac{d\omega}{2\pi}\int' \frac{d^d\boldsymbol{q}}{(2\pi)^d}\frac{e^2}{|\boldsymbol{q}|^{d-1}}\left[-\frac{i(\Omega-\omega) + v_\alpha\sum_{j=1}^d |k_j-q_j|^\alpha \mathrm{sgn}(k_j-q_j)\Gamma_j}{(\Omega-\omega)^2 + v_\alpha^2\sum_{j=1}^d|k_j-q_j|^{2\alpha}}\right]\\ &= -\frac{e^2}{2}\int' \frac{d^d\boldsymbol{q}}{(2\pi)^d}\left[\frac{v_\alpha\sum_{j=1}^d|k_j-q_j|^\alpha\mathrm{sgn}(k_j-q_j)\Gamma_j}{v_\alpha\left[\sum_{j=1}^d|k_j-q_j|^{2\alpha}\right]^{1/2}}\right].\end{aligned} \tag{S21}$$

To the leading order in the components of the momentum, it reads

$$\Sigma_d(i\Omega,\boldsymbol{k}) = k_\rho\left(\frac{\partial\Sigma_d(i\Omega,\boldsymbol{k})}{\partial k_\rho}\right)_{\boldsymbol{k}=0}. \tag{S22}$$

After some straightforward algebra we obtain

$$\left(\frac{\partial\Sigma_d(i\Omega,\boldsymbol{k})}{\partial k_\rho}\right)_{\boldsymbol{k}=0} = -\left(\frac{e^2\alpha}{h_d}\right)\Gamma_\rho\left(\int_{\Lambda e^{-\ell}}^{\Lambda}\frac{dq}{q}\right)F_{\rho,d}(\alpha) = -\left(\frac{e^2}{h_d}\right)\Gamma_\rho\,\ell\,F_{\rho,d}(\alpha), \tag{S23}$$

where $h_2 = 8\pi$, $h_3 = 6\pi^2$, and

$$F_{\rho,d}(\alpha) = \frac{\alpha}{i_d}\int d\hat{\Omega}\,|\hat{\Omega}_\rho|^{\alpha-1}\left[f(\hat{\Omega})\right]^{-1/2}\left[1 - |\hat{\Omega}_\rho|^{2\alpha}[f(\hat{\Omega})]^{-1}\right], \tag{S24}$$

with $i_2 = \pi$ and $i_3 = 8\pi/3$. We also find that $F_{\rho,d}(\alpha) \equiv F_d(\alpha)$ (independent of the component $\rho$). Therefore, when $\alpha \neq 1$ the long-range Coulomb interaction generates conventional Dirac like dispersion with $\alpha = 1$ for which the Fermi velocity ($v_1$) increases logarithmically according to

$$\frac{dv_1}{d\ell} = \frac{\alpha_{\mathrm{FS}}}{h_d}\,v_1\,F_d(\alpha), \tag{S25}$$

where $\alpha_{\mathrm{FS}} = e^2/v_1$ is the fine structure constant for conventional Dirac fermions. By contrast, the original fractional Dirac fermion dispersion remains unrenormalized due to its nonanalytic structure. The scaling of the function $F_d(\alpha)$ in $d = 2$ and $d = 3$ are shown in Fig. 3(c) and (d) of the main manuscript, with $F_2(1) = F_3(1) = 1$.

In two dimensions electronic charge does not get renormalized due to the nonanalytic structure of the photon propagator. But, in three dimensions electronic charge suffers dynamic screening due to quantum many body effects, which is captured by the polarization bubble given by

$$\Pi(i\Omega,\boldsymbol{k}) = -e^2\mathrm{Tr}\left[\int_{-\infty}^{\infty}\frac{d\omega}{2\pi}\int'\frac{d^3\boldsymbol{q}}{(2\pi)^3}G_0(i\omega+i\Omega,\boldsymbol{k}+\boldsymbol{q})G_0(i\omega,\boldsymbol{q})\right] = De^2\left(I_1 - I_2\right), \tag{S26}$$

obtained after carrying out the integral over the Matsubara frequency $\omega$, where

$$I_1 = \frac{1}{2v_\alpha} \int' \frac{d^3\boldsymbol{q}}{(2\pi)^3} \left[ \sum_{j=1}^{d} |(\boldsymbol{k}+\boldsymbol{q})_j|^{2\alpha} + \sum_{j=1}^{d} |\boldsymbol{q}_j|^{2\alpha} \right]^{-1},$$

$$\text{and} \quad I_2 = \frac{1}{2v_\alpha} \int' \frac{d^3\boldsymbol{q}}{(2\pi)^3} |(\boldsymbol{k}+\boldsymbol{q})_j|^{\alpha-1} |\boldsymbol{q}_j|^{\alpha-1} (\boldsymbol{k}+\boldsymbol{q})_j (\boldsymbol{q})_j \times \left[ \sum_{j=1}^{d} |(\boldsymbol{k}+\boldsymbol{q})_j|^{2\alpha} + \sum_{j=1}^{d} |\boldsymbol{q}_j|^{2\alpha} \right]^{-1} \left[ \sum_{j=1}^{d} |(\boldsymbol{k}+\boldsymbol{q})_j|^{2\alpha} \right]^{-1/2} \left[ \sum_{j=1}^{d} |\boldsymbol{q}_j|^{2\alpha} \right]^{-1/2}. \tag{S27}$$

The logarithmically divergent piece of the polarization bubble yielding charge renormalization reads as

$$\Pi_{\rho\sigma}(0,\boldsymbol{k}) = \frac{D}{2} k_\rho k_\sigma \left[ \left( \frac{\partial^2 I_1}{\partial k_\rho \partial k_\sigma} \right)_{\boldsymbol{k}=0} - \left( \frac{\partial^2 I_2}{\partial k_\rho \partial k_\sigma} \right)_{\boldsymbol{k}=0} \right] \frac{e^2}{v_\alpha \Lambda^{\alpha-1}} \ \ell, \tag{S28}$$

where $\rho, \sigma = 1, 2, 3$ are the spatial indices. After some straightforward otherwise tedious algebra, we obtain

$$\left( \frac{\partial^2 I_1}{\partial k_\rho \partial k_\sigma} \right)_{\boldsymbol{k}=0} = \frac{\alpha}{8}(\alpha+1) I_{\rho\sigma} - \frac{\alpha}{8}(2\alpha-1)\delta_{\rho\sigma} J_\rho \ \text{and} \ \left( \frac{\partial^2 I_2}{\partial k_\rho \partial k_\sigma} \right)_{\boldsymbol{k}=0} = \frac{\alpha^2}{2} I_{\rho\sigma} + \frac{\alpha}{8}(1-4\alpha)\delta_{\rho\sigma} J_\rho, \tag{S29}$$

where

$$J_\rho(\alpha) = \int \frac{d\hat{\Omega}}{(2\pi)^3} \frac{|\hat{\Omega}_\rho|^{2\alpha-2}}{[f(\hat{\Omega})]^{3/2}} \equiv J(\alpha) \ \text{and} \ I_{\rho\sigma} = \int \frac{d\hat{\Omega}}{(2\pi)^3} \frac{|\hat{\Omega}_\rho|^{2\alpha-2} |\hat{\Omega}_\sigma|^{2\alpha-2} \hat{\Omega}_\rho \hat{\Omega}_\sigma}{[f(\hat{\Omega})]^{5/2}} \equiv I(\alpha) \delta_{\rho\sigma}. \tag{S30}$$

Collecting all the terms we can write the polarization bubble compactly as

$$\Pi_{\rho\sigma}(0,\boldsymbol{k}) = \frac{D}{4} \frac{\alpha}{4} \alpha_{\rm FS} \ k_\rho k_\sigma \delta_{\rho\sigma} \ [(1-3\alpha) I(\alpha) + 2\alpha J(\alpha)] \ \ell, \tag{S31}$$

which leads to the RG flow equation for the electric charge in three-dimensional FDMs shown in Eq. (14) of the main manuscript, where the results are quoted for $D = 4$.
